# Supplementary material for: Self-Supervised Generation of Spatial Audio for 360 Video
Source: arXiv:1809.02587 source file (2018-09-07)
Supplement: Supplementary file 1 [file appendix.tex]

\begin{figure}[t!]
	\centering
	\includegraphics[width=0.8\linewidth]{figures/audio-enc.pdf}
	\caption{\label{fig:audio_enc}\textbf{Audio encoder}. Detailed representation of audio encoder architecture. Forward pass is left to right.}
\end{figure}
\begin{figure}[t!]
	\centering
	\includegraphics[width=0.8\linewidth]{figures/sep-network.pdf}
	\caption{\label{fig:sep_net}\textbf{Separation}. Detailed representation of source separation architecture. Forward pass is left to right.}
\end{figure}
\begin{figure}[t!]
	\centering
	\includegraphics[width=0.5\linewidth]{figures/loc-network.pdf}
	\caption{\label{fig:loc_net}\textbf{Localization}. Detailed representation of localization architecture. Forward pass is left to right.}
\end{figure}

\appendix
\section{Appendix}
\subsection{Network Architectures}
\label{appx:architecture}
Both video and flow encoders use the ResNet-18 architecture up to the last convolutional layer. Then, a 1x1 convolutional layer reduces the dimensionality of the feature maps to 128, and a fully-connected layer is used to compute from the resulting map of size 7x14x128, a 512-dimensional global feature vector.
Flow features are extracted from the X and Y displacements, as well as the magnitude of the corresponding velocity vector. 
The audio encoder is a 5 layer CNN applied to the input STFT and detailed in Fig.~\ref{fig:audio_enc}. 
%It outputs a 256 dimensional feature representation of the audio that is concatenated to the both video and flow features. 

The concatenated audio and video features are then fed to the separation and localization blocks, shown in Figs.~\ref{fig:sep_net} and \ref{fig:loc_net}, respectively. 
The separation net outputs the $k=32$ frequency activation maps to be used for modulation of the input STFT, and separated wave-forms $f^{i}(t)$ are computed by inverse STFT. In our implementation, the number of frequency components is $1024$.
The localization net outputs, for each of the $k=32$ sources, the 3 localization weights ${\bf w}^{i}$ associated with the three ambisonics channels ${\pmb\phi}=(\phi_x, \phi_y, \phi_z)$. 

Given the localization weights ${\bf w}^{i}(t)$ and separated wave-forms $f^{i}(t)$, the FOA are generated by 
$$\textstyle{\pmb\phi}(t)=\sum_{i=1}^k {\bf w}^{i}(t)f^{i}(t).$$

%\begin{figure}[ht]
%	\centering
%	\includegraphics[width=0.7\linewidth]{figures/id_net.pdf}
%	\caption{\label{fig:id_net}\textbf{Analysis}. Detailed representation of \textsc{AnalysisNet}.}
%\end{figure}
%
%\begin{figure}[ht]
%	\centering
%	\includegraphics[width=0.7\linewidth]{figures/separation_net.pdf}
%	\caption{\label{fig:sep_net}\textbf{Separation}. Detailed representation of \textsc{SeparationNet}.}
%\end{figure}
%
%\begin{figure}[ht]
%	\centering
%	\includegraphics[width=0.7\linewidth]{figures/localization_net.pdf}
%	\caption{\label{fig:loc_net}\textbf{Localization}. Detailed representation of \textsc{LocalizationNet}.}
%\end{figure}
%
%\begin{figure}[p]
%	\centering
%	\includegraphics[width=\linewidth]{figures/network-details.pdf}
%	\caption{\label{fig:net_details}\textbf{Network details}. Detailed representation of \textsc{AnalysisNet}, \textsc{SeparationNet} and \textsc{LocalizationNet}.}
%\end{figure}

%
%\paragraph{U-Net}
%\pmm{Needed?  There's already a good description before.}
